# Supplementary material for: Critical decay exponent of the pair contact process with diffusion
Source: arXiv:1202.6024 source file (2014-11-21)
Supplement: Supplementary file 1 [file supp.pdf]

# Supplemental Material for “Critical decay exponent of the pair contact process with diffusion”

Su-Chan Park

*Department of Physics, The Catholic University of Korea,  
Bucheon 420-743, Republic of Korea*

## Abstract

In this Supplemental Material (SM), we present more figures to support the claim in the main text. The appearance order of figures in the SM is the same as the order mentioned in the main text.

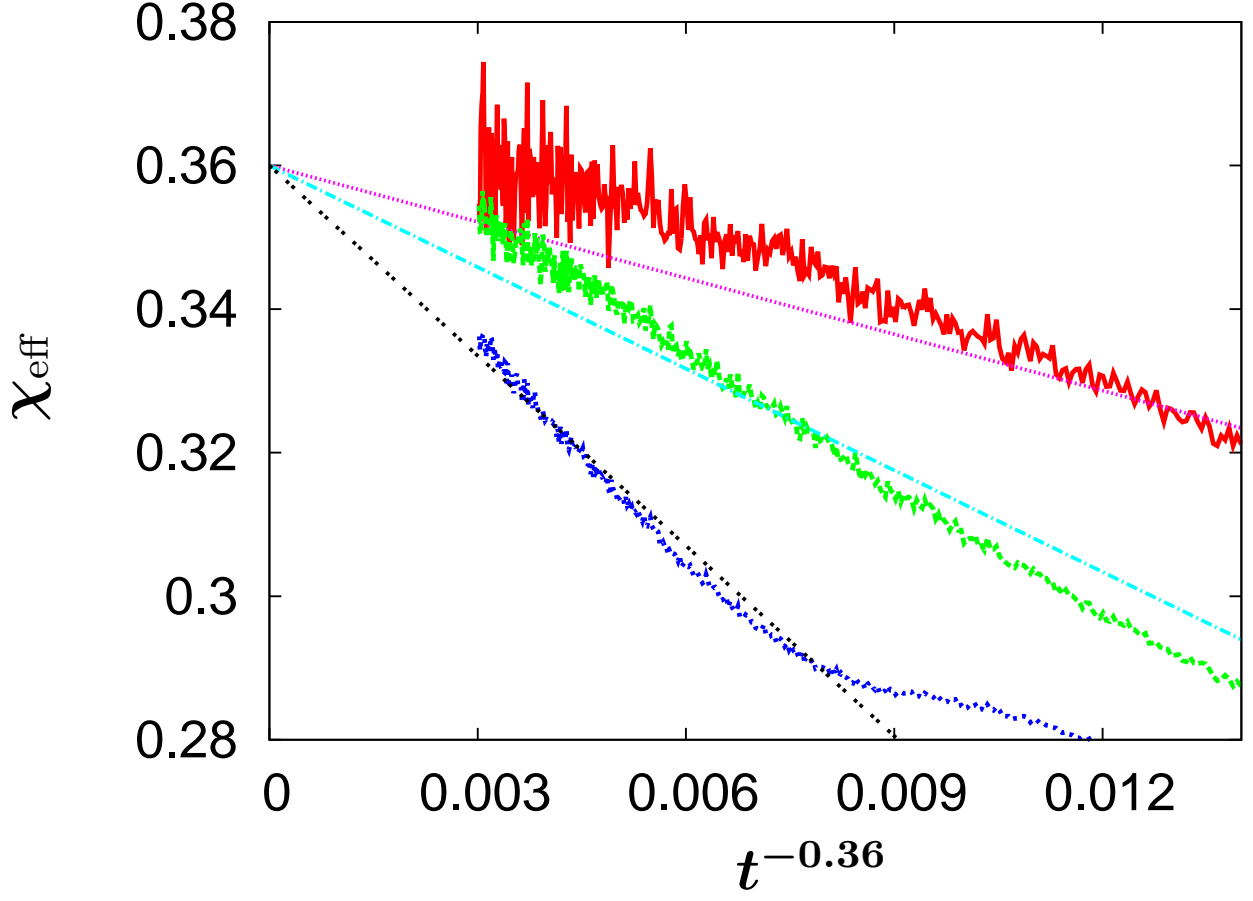

**SM Fig. 1.** (Color online) Plots of  $\chi_{\text{eff}}(t; b)$  for  $b = 10^{3/2}$  (top curve),  $b = 10^2$  (middle curve), and  $b = 10^{5/2}$  (bottom curve) as functions of  $t^{-0.36}$ . The straight lines are resulting fitting functions using  $\chi = 0.36$  obtained from the process explained in Sec. III A. This figure should be compared with Fig. 1 in the main text.

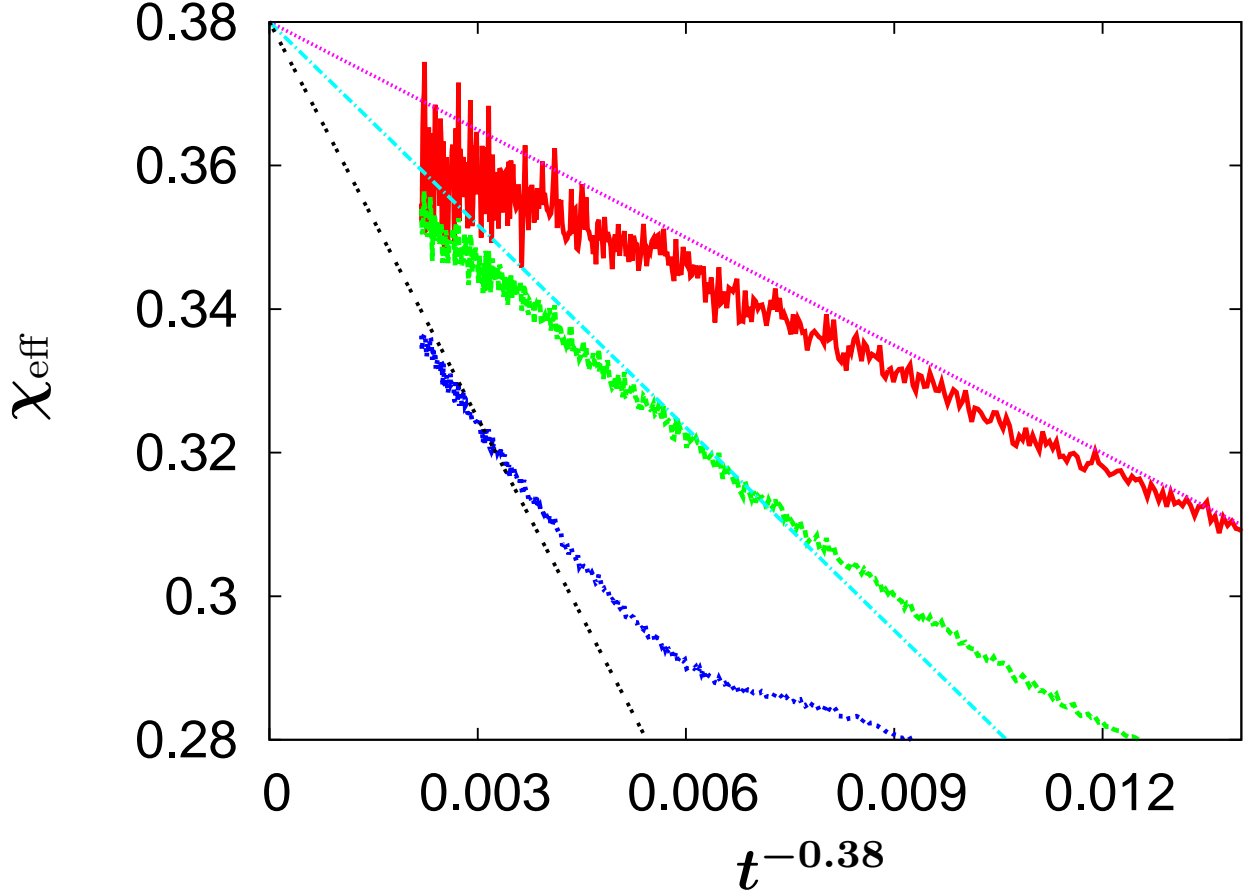

**SM Fig. 2.** (Color online) Plots of  $\chi_{\text{eff}}(t; b)$  for  $b = 10^{3/2}$  (top curve),  $b = 10^2$  (middle curve), and  $b = 10^{5/2}$  (bottom curve) as functions of  $t^{-0.38}$ . The straight lines are resulting fitting functions using  $\chi = 0.38$  obtained from the process explained in Sec. III A. This figure should be compared with Fig. 1 in the main text. This figure together with **SM Fig. 1** is used to assign the error of  $\chi$  in the main text.

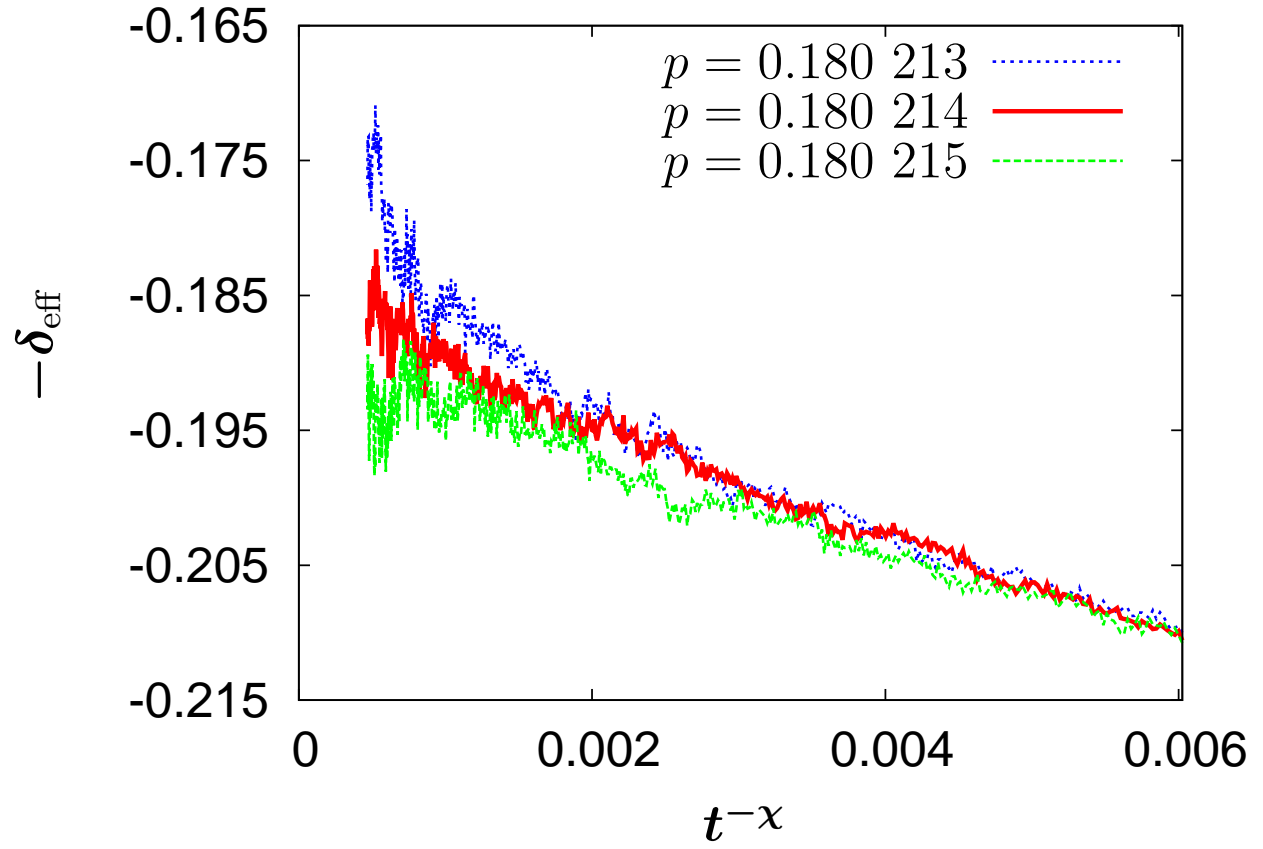

**SM Fig. 3.** Effective exponent of the pair density obtained using  $b = 100$ . This figure should be compared to Fig. 2 of the main text.

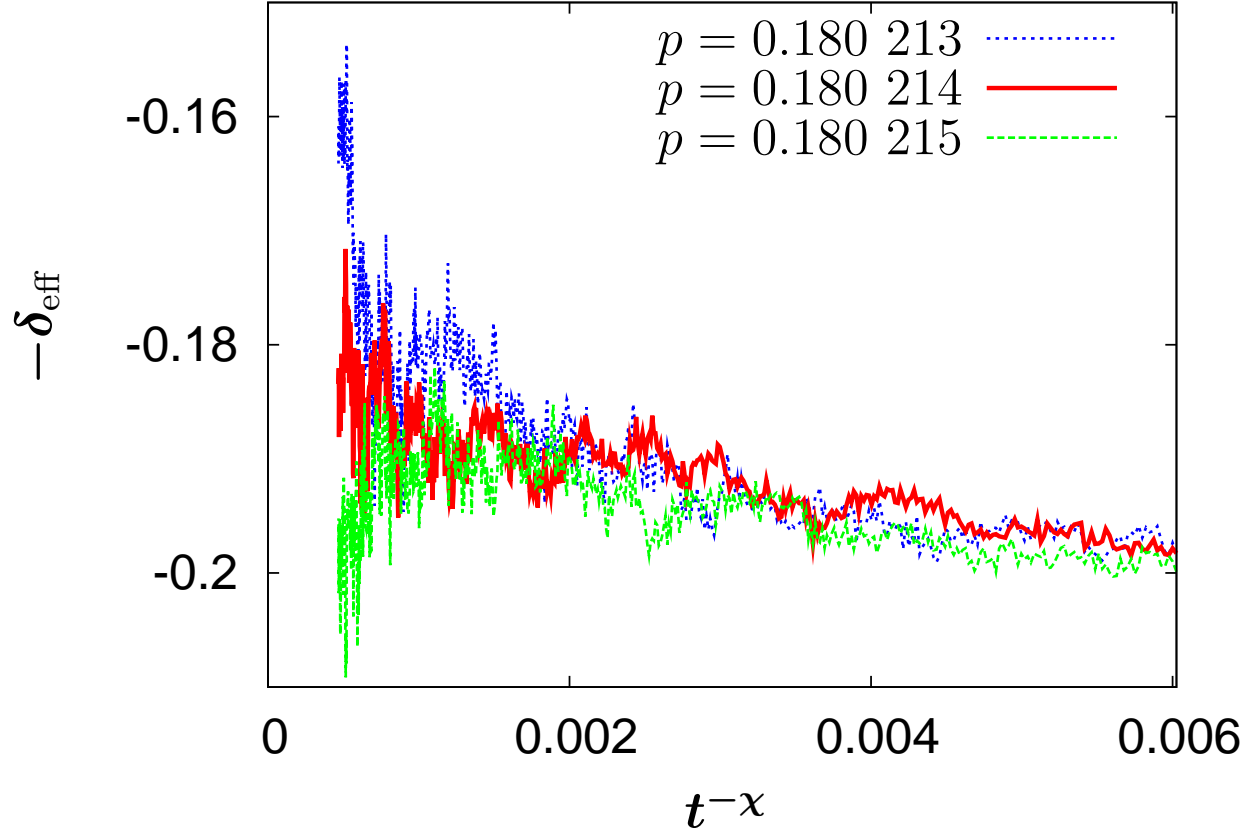

**SM Fig. 4.** Effective exponents of the particle density obtained using  $b = 10$ . In particular,  $-\delta_{\text{eff}}$  for  $p = 0.180\ 215$  shows a significant curvature, compared to Fig. 2 of the main text.

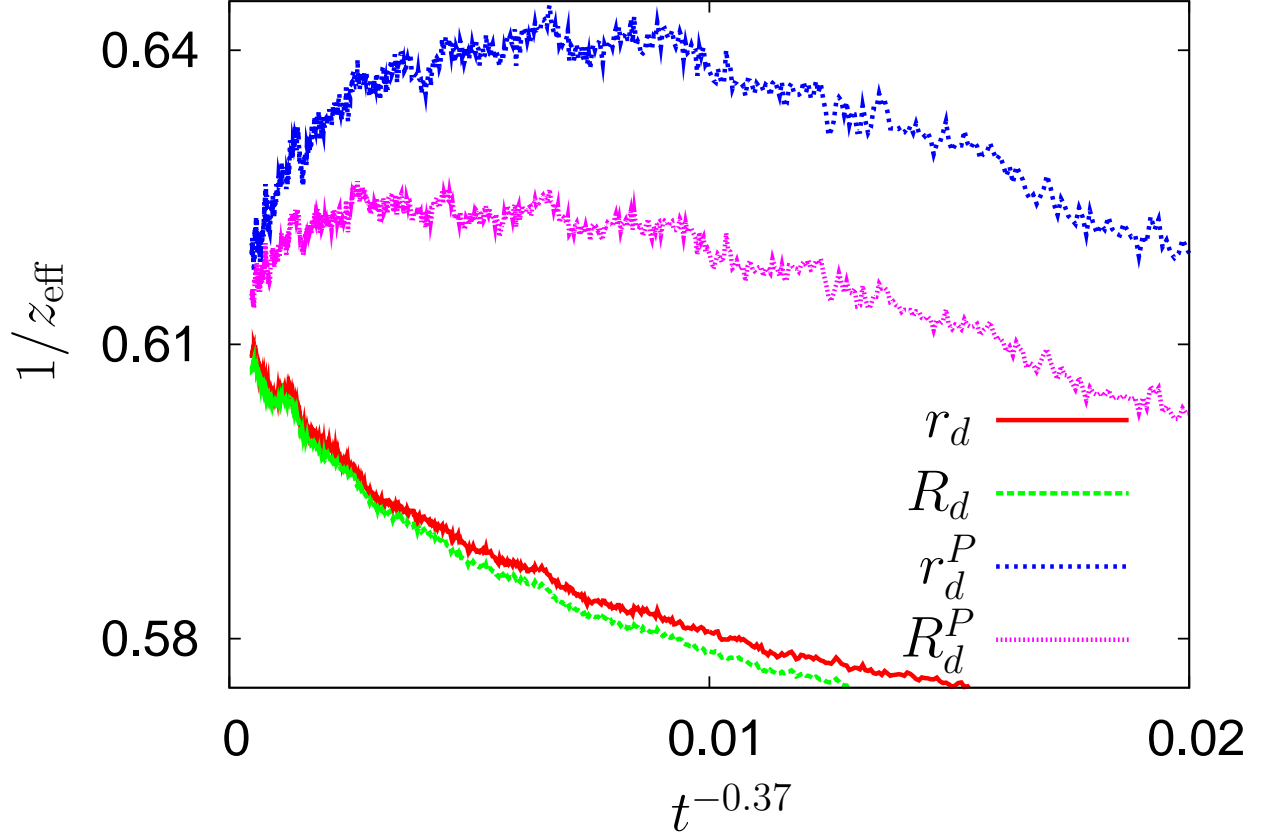

**SM Fig. 5.** Effective exponents for  $1/z_d$  obtained from  $r_d$ ,  $R_d$ ,  $r_d^P$ , and  $R_d^P$  of the PCPD within the D-ensemble scheme. All curves approach to the same value  $\approx 0.61$  as  $t^{-0.37} \rightarrow 0$ . This figure is associated with Fig. 10 of the main text.

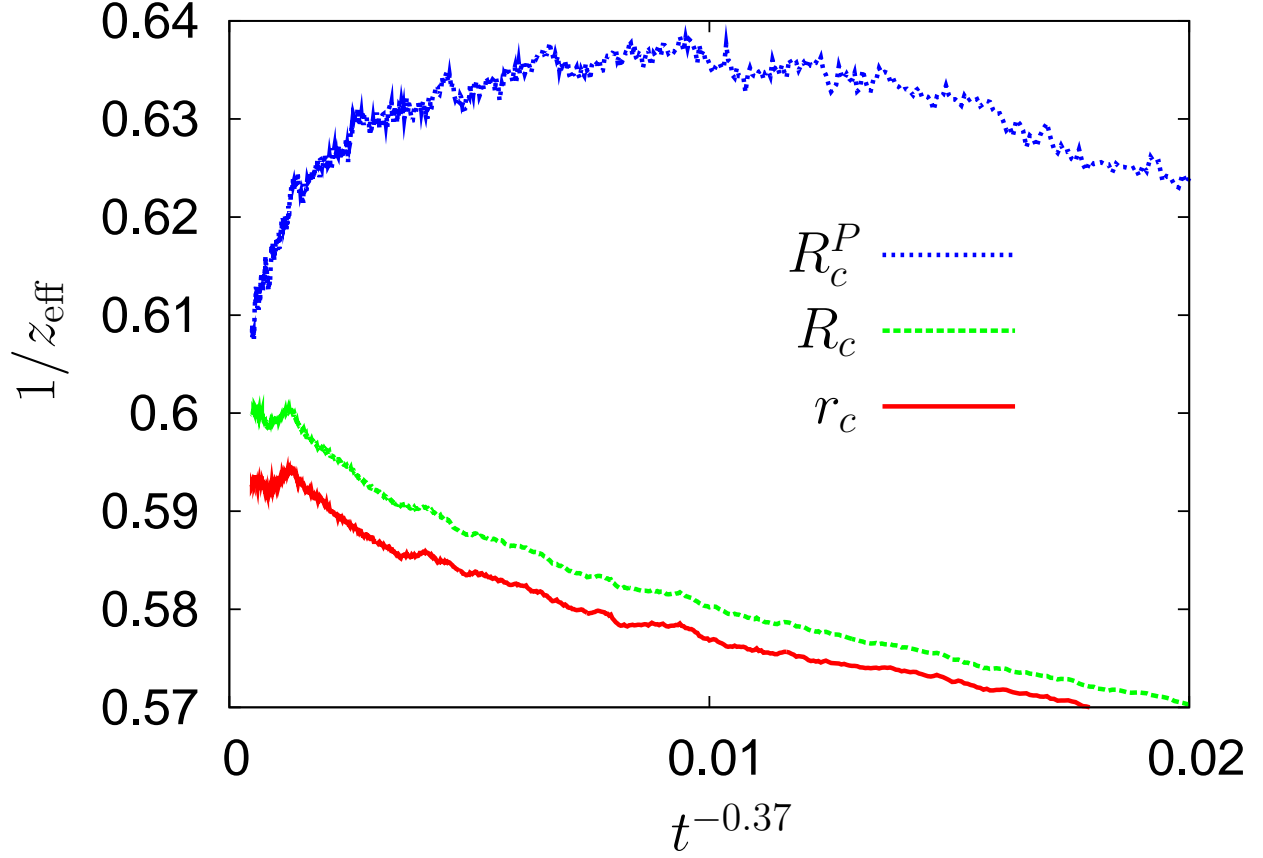

**SM Fig. 6.** Effective exponents for  $1/z_c$  obtained from  $r_c$ ,  $R_c$ , and  $R_c^P$ . First note that the effective exponents for  $R_c$  and  $R_c^P$  both approach to 0.6 rather than 0.61. Second note that the effective exponent for  $r_c$  even does not approach to 0.6. This figure supports the claim in the main text that  $z_c$  is ill-defined.

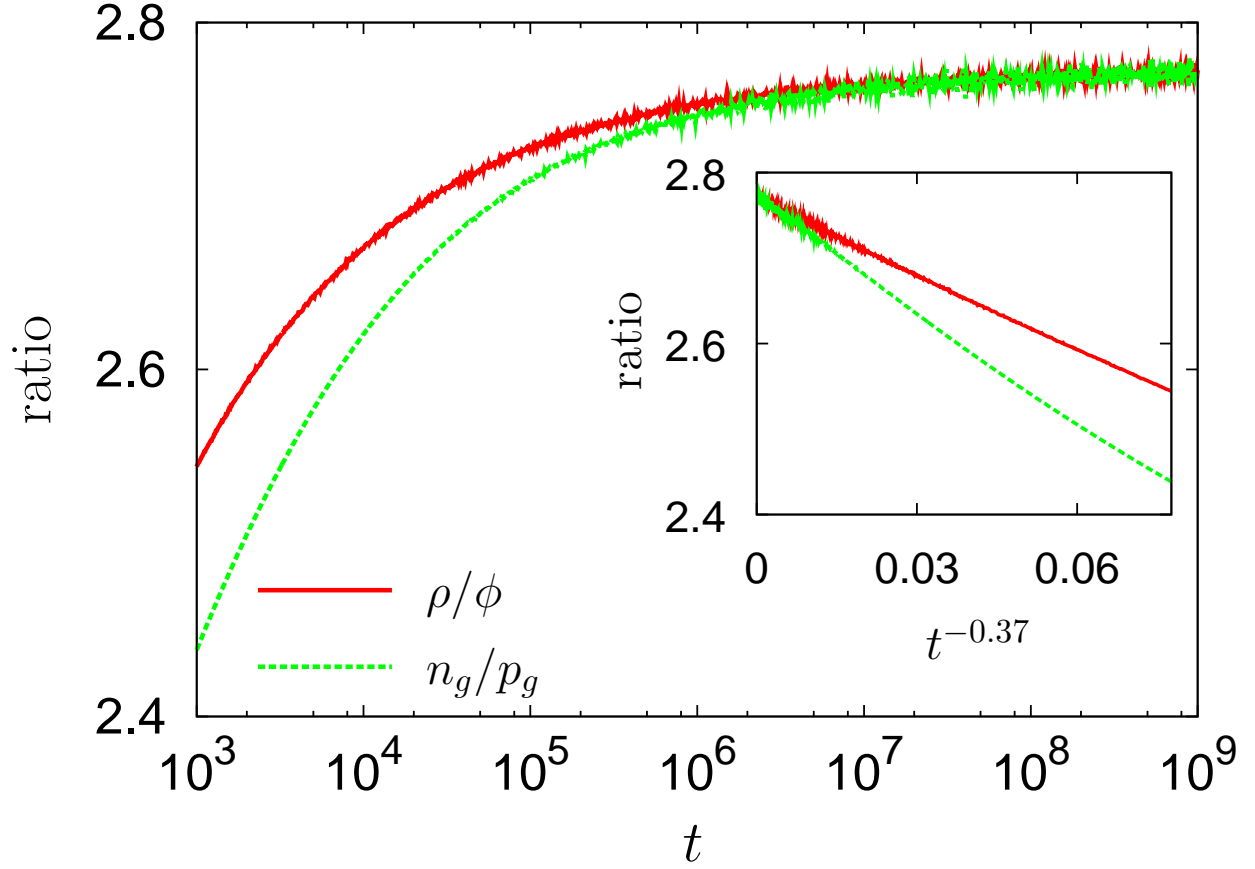

**SM Fig. 7.** Log-log plots of  $\rho/\phi$  and  $n_g/p_g$  for the PCPD as functions of  $t$ . After  $t = 10^7$ , the difference between two curves are hardly detectable. Inset: Plots of  $\rho/\phi$  and  $n_g/p_g$  as functions of  $t^{-0.37}$  on a linear scale. Both curves show a linear approach to the ordinate, which supports that the leading correction to scaling is  $t^{-0.37}$ . This figure is pertinent to Inset of Fig. 12 and the corresponding discussion in the main text.
